# Supplementary material for: Feature Distribution Shift Mitigation with Contrastive Pretraining for Intrusion Detection
Source: arXiv:2404.15382 source file (2024-04-23)
Supplement: Supplementary file 1 [file 09_appendix.tex]

\label{sec:appendix}
